# Supplementary material for: Boltzmann priors for Implicit Transfer Operators
Source: arXiv:2410.10605 source file (2025-04-02)
Supplement: Supplementary file 1 [file ito_appendix.tex]

\section{Properties of the Transfer operator}

\subsection{Relaxation of $T_\Omega$ spectrum \label{app:omegaspectrum}}
In this section, we outline the `relaxation' or `decay' of the spectral components of $T_\Omega$ as a function of time-step, $\tau$. We use that $\langle \phi_i| \psi_i \rangle_\mu= \int \phi_i(x) \psi_i(x)\,  \mathrm{d}\mu(x) =1$ if $i=j$ and $0$ if $i\neq j$, e.g. the eigenfunctions are orthonormal under the $\mu$-weighed inner-product. Since $T_\Omega(\tau)$ is Markov, composing $T_\Omega(\tau)$ with itself $N$ times we get,
\begin{eqnarray}
    [T_\Omega(\tau)]^N &=& T_\Omega(\tau)\circ \dots \circ T_\Omega(\tau) \\
    &=& \sum_{i=0}^\infty \lambda_i(\tau) | \psi_i \rangle \langle \phi_i|\lambda_i(\tau) | \psi_i \rangle \langle \phi_i| \dots \lambda_i(\tau) | \psi_i \rangle \langle \phi_i|\\
    &=& \sum_{i=0}^\infty \lambda_i(\tau)^N | \psi_i \rangle \langle \phi_i| \psi_i \rangle_\mu \langle \phi_i|\dots | \psi_i \rangle \langle \phi_i| \\
    &=& \sum_{i=0}^\infty \lambda_i(\tau)^N | \psi_i \rangle \langle\phi_i |
\end{eqnarray}

We assume the dynamics governed by $T_\Omega$ are
\begin{enumerate}
    \item reversible $\lambda_i \in \mathbb{R}$
    \item measure-preserving  $0\leq |\lambda_i| \leq 1$
    \item ergodic, $\lambda_0=1$ and $|\lambda_{i>0}| < 1$
\end{enumerate}
 where we have sorted the eigenvalues eigenfunction pairs in descending order. Consequently, for $N\rightarrow \infty$ we have $T_\Omega(N\tau) \rightarrow | \mathbb{1}\rangle \langle \mu| $, where $\mathbb{1}$ is the constant function. 

\subsection{Decomposition of transition density \label{app:transitiondensity}}
In this section, we detail the decomposition of the transition density, $p(\mathbf{x}_{N\tau}\mid \mathbf{x}_0)$.

Let $\rho$ specify an initial condition, an absolutely convergent probability density function on $\Omega$. We can define a Transfer operator $T_{\Omega}$ using a transition probability density \cite{schutte2009conformation}:
\begin{eqnarray}
    \left[T_{\Omega}\circ \rho\right] (\mathbf{x}_{N\tau}) \triangleq  \frac{1}{\mu(\mathbf{x}_{N\tau})}\int_{\mathbf{x}_0}\mu(\mathbf{x}_0)\rho(\mathbf{x}_0)p(\mathbf{x}_{N\tau}\mid \mathbf{x}_0)\, \mathrm{d}\mathbf{x}_0, \hspace{0.5cm}  T_{\Omega}: L^1 (\Omega) \rightarrow L^1(\Omega)
\end{eqnarray}

which then describes the $\mu$-weighed evolution of densities on $\Omega$ according to MD discretized in time by a step-size of $\tau$. $\mu$ is a normalized Gibbs measure, or the Boltzmann distribution. 

Since we only consider MD with time-invariant drift, only the eigenvalues $\lambda_i(\tau)$ of $T_\Omega(\tau)$ depend on $\tau$. We can express arbitrary transition probabilities through a bilinear form
\begin{equation}
p(\mathbf{x}_{N\tau}\mid \mathbf{x}_0) = \langle \delta_{\mathbf{x}_{N\tau}}| T_\Omega^N(\tau) | \delta_{\mathbf{x}_0} \rangle  = \sum_{i=1}^{\infty} \lambda_i^N(\tau)\langle \delta_{\mathbf{x}_{N\tau}}|\phi_i\rangle\langle \psi_i| \delta_{\mathbf{x}_0} \rangle = \sum_{i=1}^\infty \lambda_i^N(\tau) \alpha_i(\mathbf{x}_{N\tau})\beta_i(\mathbf{x}_0) \label{eq:tprob_long}
\end{equation}
where $\alpha_i$ and $\beta_i$ are {\it time-invariant} projections coefficients of the state variables on-to the eigenfunctions $\phi_i$ and $\psi_i$, and $\delta_{\mathbf{x}}$ is the Dirac delta centered at $\mathbf{x}$. $T_\Omega^N(\tau)$ means $T_\Omega(\tau)$ acting $N$ times (See \ref{app:omegaspectrum}).
